# Supplementary material for: [Vision Paper] PRObot: Enhancing Patient-Reported Outcome Measures for Diabetic Retinopathy using Chatbots and Generative AI
Source: arXiv:2411.02973 source file (2024-11-05)
Supplement: Supplementary file 1 [file appendix.tex]

\label{appendix}
